# Supplementary material for: Cram\'er-Rao Bounds for Holographic Positioning
Source: arXiv:2111.02229 source file (2022-11-03)
Supplement: Supplementary file 1 [file AppendixE.tex]

 %!TEX root = main.tex
\section*{Appendix E}
\label{app:MFelem}

EXPLICIT FORM FOR THE FISHER'S MATRIX COMPONENTS

\subsection{Ft}

We now compute the elements of $\mathbf{F}_t$. 

\begin{align}
\label{Ft11}\notag
[\mathbf{F}_t]_{11}&=\dfrac{1}{\sigma^2}\iint_{-L/2}^{L/2} \left[\left|\derpar{E_x}{t_x}\right|^2+\left|\derpar{E_y}{t_x}\right|^2+\left|\derpar{E_z}{t_x}\right|^2\right]dy dz\\
&=\dfrac{|\chi|^2}{\sigma^2}\iint_{-L/2}^{L/2} \dfrac{1-r_x^2}{r^2}dy dz=\dfrac{|\chi|^2}{\sigma^2}\iint_{-L/2}^{L/2} \dfrac{y^2+z^2}{r^4}dy dz
\end{align}

This integral does not admit a close form, but we can easily provide an upper and lower bound.
%Tale integrale non si riesce ad esprimere in forma chiusa. si possono, per\`o, calcolare facilmente un \textit{bound} inferiore ed uno superiore dati da

\begin{align}
\label{LB_Ft_11}
LB\big([\mathbf{F}_t]_{11}\big)=\dfrac{\pi |\chi|^2}{\sigma^2} \left[ \ln(1+\rho^2)-\dfrac{\rho^2}{1+\rho^2} \right]
\end{align}

\begin{align}
\label{UB_Ft_11}
UB\big([\mathbf{F}_t]_{11}\big)=\dfrac{\pi |\chi|^2}{\sigma^2} \left[ \ln(1+2\rho^2)-\dfrac{2\rho^2}{1+2\rho^2} \right]
\end{align}
for $\rho=L/x_s$.

\begin{align}
\label{Ft22}\notag
[\mathbf{F}_t]_{22}&=\dfrac{1}{\sigma^2}\iint_{-L/2}^{L/2} \left[\left|\derpar{E_x}{t_y}\right|^2+\left|\derpar{E_y}{t_y}\right|^2+\left|\derpar{E_z}{t_y}\right|^2\right]dy dz\\
&=\dfrac{|\chi|^2}{\sigma^2}\iint_{-L/2}^{L/2} \dfrac{1-r_y^2}{r^2}dy dz=\dfrac{|\chi|^2}{\sigma^2}\iint_{-L/2}^{L/2} \dfrac{x_s^2+z^2}{r^4}dy dz
\end{align}

Even in this case, the integral can not be solved, but we can find an upper and lower bound given by
%Anche in questo caso l'integrale non si riesce a calcolare in forma chiusa, ma si trovano un \textit{bound} inferiore ed uno superiore dati da

\begin{align}
\label{LB_Ft_22}
LB\big([\mathbf{F}_t]_{22}\big)=\dfrac{|\chi|^2}{\sigma^2} \dfrac{4 \rho}{\sqrt{1+\rho^2}}\arctan\dfrac{\rho}{\sqrt{1+\rho^2}}+\dfrac{1}{2} LB\big([\mathbf{F}_t]_{11}\big)
\end{align}

\begin{align}
\label{UB_Ft_22}
UB\big([\mathbf{F}_t]_{22}\big)=\dfrac{|\chi|^2}{\sigma^2} \dfrac{4 \rho}{\sqrt{1+\rho^2}}\arctan\dfrac{\rho}{\sqrt{1+\rho^2}}+\dfrac{1}{2} UB\big([\mathbf{F}_t]_{11}\big)
\end{align}

\begin{align}
\label{Ft23}\notag
[\mathbf{F}_t]_{23}&=\dfrac{1}{\sigma^2}\iint_{-L/2}^{L/2} \left[\derpar{E_x}{t_y}\derpar{E^\ast_x}{t_z}+\derpar{E_y}{t_y}\derpar{E^\ast_y}{t_z}+\derpar{E_z}{t_y}\derpar{E^\ast_z}{t_z}\right]dy dz\\
&=-\dfrac{|\chi|^2}{\sigma^2}\iint_{-L/2}^{L/2} \dfrac{r_y r_z}{r^2}dy dz=0
\end{align}

\begin{align}
\label{Ft33}\notag
[\mathbf{F}_t]_{33}&=\dfrac{1}{\sigma^2}\iint_{-L/2}^{L/2} \left[\left|\derpar{E_x}{t_z}\right|^2+\left|\derpar{E_y}{t_z}\right|^2+\left|\derpar{E_z}{t_z}\right|^2\right]dy dz\\\notag
&=\dfrac{|\chi|^2}{\sigma^2}\iint_{-L/2}^{L/2} \dfrac{1-r_z^2}{r^2}dy dz=\dfrac{|\chi|^2}{\sigma^2}\iint_{-L/2}^{L/2} \dfrac{x_s^2+y^2}{r^4}dy dz\\
&=[\mathbf{F}_t]_{22}
\end{align}

Equations \eqref{Ft11}--\eqref{Ft33} shows that, under the CPL hypothesis, matrix $\mathbf{F}_t$ is diagonal.

%Le equazioni mostrano che,  quando vale l'ipotesi CPL, anche la matrice \`e una matrice diagonale.
